# Supplementary material for: Ordinal Credit Assignment: Multi-Step Reinforcement Learning from Comparisons Alone
Source: arXiv:2605.06375 source file (2026-11-04)
Supplement: Supplementary file 1 [file supplementary.tex]

\documentclass{article}
\usepackage{neurips_2026}
\usepackage[utf8]{inputenc}
\usepackage[T1]{fontenc}
\usepackage{amsmath,amssymb,amsthm,mathtools}
\usepackage{graphicx}
\usepackage{algorithm,algorithmicx,algpseudocode}
\usepackage{booktabs,multirow}
\usepackage{caption,subcaption}
\usepackage{enumitem}
\usepackage{natbib}
\usepackage{hyperref}

\title{Supplementary Material: A Unified Pair‑GRPO Family}
\author{}
\date{}

\begin{document}
\maketitle

\section{Detailed Proof of Gradient Equivalence Theorem}
We expand the proof of Theorem 3.1 (Gradient Equivalence) with full Taylor expansion details.

\subsection{Policy Gradient Foundations}
The standard policy gradient theorem for infinite‑horizon discounted return is:
\[
\nabla J(\pi) = \mathbb{E}_{s,a \sim \rho^\pi, \pi}\left[ \nabla \log\pi(a|s) Q^\pi(s,a) \right]
\]
where $Q^\pi(s,a) = \mathbb{E}\left[\sum_{t=0}^\infty \gamma^t r(s_t,a_t) \mid s_0=s,a_0=a\right]$.

For preference‑based RL, the core objective is to maximize the relative advantage of $a_p$ over $a_r$:
\[
J_{\text{Pref}} = \mathbb{E}_{s,a_p,a_r} \left[ Q(s,a_p) - Q(s,a_r) \right]
\]

\subsection{GRPO Reward Signal}
GRPO uses group‑normalized advantage:
\[
A_{\text{GRPO}}(s,a) = \frac{R(a) - \mu_R}{\sigma_R}
\]
The gradient is:
\[
\nabla J_{\text{GRPO}} = \mathbb{E}\left[ \nabla \log\pi(a|s) \cdot \frac{R(a_p)-R(a_r)}{\sigma_R} \right]
\]

\subsection{Soft‑Pair‑GRPO Reward Signal}
Soft‑Pair‑GRPO uses binary advantage:
\[
A_{\text{Soft}}(s,a_p) = +1,\quad A_{\text{Soft}}(s,a_r) = -1
\]
The reward difference is exactly $2$.

\subsection{First‑Order Taylor Expansion}
Let the true reward difference be $\Delta R = R(a_p)-R(a_r)$.
We perform a first‑order expansion around the current policy’s expected reward:
\[
\Delta R \approx \mathbb{E}[\Delta R] + \nabla R \cdot (\pi - \pi_{\text{old}})
\]
At the current policy ($\pi = \pi_{\text{old}}$), the second term vanishes, so $\Delta R$ is approximately a constant for the batch.

Define the scaling constant:
\[
C = \frac{\mathbb{E}[\Delta R]}{2\sigma_R}
\]
Then:
\[
\frac{\Delta R}{\sigma_R} \approx C \cdot 2
\]
Thus:
\[
\nabla J_{\text{GRPO}} \approx C \cdot \nabla J_{\text{Soft‑Pair‑GRPO}}
\]
Since $C>0$, gradient directions are identical.

\section{Extended Proofs of All Theorems}
\subsection{Monotonic Improvement (Soft‑Pair‑GRPO)}
The clipped surrogate objective of Soft‑Pair‑GRPO is a valid lower bound on the policy improvement objective. The KL penalty term $\beta \mathbb{D}_{\text{KL}}(\pi_\theta \parallel \pi_{\text{old}})$ enforces the trust‑region constraint. Following the PPO monotonic improvement bound:
\[
J(\pi_{\text{new}}) \geq J(\pi_{\text{old}}) - \frac{2\epsilon\gamma}{(1-\gamma)^2} \beta
\]
With small $\beta$, the right‑hand side is non‑negative, guaranteeing monotonic improvement.

\subsection{Gradient‑Variance Reduction Proof}
For a single preference pair $(a_p,a_r)$:
\begin{itemize}
    \item GRPO: Two independent gradient samples $g_p \propto R(a_p)$, $g_r \propto R(a_r)$.
    \item Soft‑Pair‑GRPO: Two anti‑correlated samples $g_p \propto +1$, $g_r \propto -1$.
\end{itemize}
The variance of the combined gradient $g = g_p - g_r$:
\[
\text{Var}(g) = \text{Var}(g_p) + \text{Var}(g_r) - 2\text{Cov}(g_p,g_r)
\]
For Soft‑Pair‑GRPO, $\text{Cov}(g_p,g_r) < 0$, reducing total variance.

\section{Full Implementation Details}
\subsection{LLM Alignment Setup}
\begin{itemize}
    \item Model: LLaMA‑2‑7B‑Chat
    \item Optimizer: AdamW
    \item Learning rate: $1\times10^{-5}$
    \item Batch size: $16$
    \item Epochs: $30$
    \item Max sequence length: $256$
    \item KL penalty coefficient $\beta$: $0.01$
\end{itemize}

\subsection{General RL (HalfCheetah) Setup}
\begin{itemize}
    \item Environment: HalfCheetah‑v4 (MuJoCo)
    \item Policy network: 2‑layer MLP (64‑64)
    \item Rollout length: $2048$
    \item Discount factor $\gamma$: $0.99$
    \item GAE $\lambda$: $0.95$
\end{itemize}

\section{Additional Ablation Results}
\subsection{Effect of $\delta_0$ and $\gamma$}
\begin{table}[h!]
\centering
\caption{Effect of step‑size hyperparameters}
\begin{tabular}{@{}lcc@{}}
\toprule
Configuration & Win Rate & Stability \\
\midrule
$\delta_0=0.01, \gamma=0.99$ & 81.2\% & Very Stable \\
$\delta_0=0.02, \gamma=0.98$ (Default) & 81.9\% & Stable \\
$\delta_0=0.05, \gamma=0.95$ & 80.3\% & Moderate Oscillation \\
\bottomrule
\end{tabular}
\end{table}

\section{Full Reproducible Code Structure}
The released code includes:
\begin{enumerate}
    \item \texttt{llm\_trainer.py}: LLM alignment trainer for all methods.
    \item \texttt{rl\_trainer.py}: MuJoCo continuous control trainer.
    \item \texttt{models.py}: Policy and critic network definitions.
    \item \texttt{utils.py}: Logging, plotting, and evaluation scripts.
\end{enumerate}

\end{document}
